# Supplementary material for: AttackBench: Evaluating Gradient-based Attacks for Adversarial Examples
Source: arXiv:2404.19460 source file (2025-05-12)
Supplement: Supplementary file 1 [file adversarial_attacks.tex]

\section{Gradient-based Attacks}

We present here an original categorization of gradient-based attacks on machine-learning models that unifies different formulations in the literature (\autoref{sec:categor}), and then discuss the main limitations present in current attack evaluations and comparisons (\autoref{sec:limitation_evaluation}).%, which we aim to overcome within our \ab framework.

\subsection{Attack Categorization}
\label{sec:categor}

Summarized in Table~\ref{table:adv_attacks_categorization}, our categorization is defined by (i) the attack type and the perturbation constraints, (ii) the loss function optimized by the attack, (iii) the initialization strategies, (iv) the descent direction used by the attack to update the perturbation in each iteration, (v) the optimization algorithm, and (vi) the scheduling policy for annealing the step size during the optimization. We present each of these aspects in the following sections.

\begin{table*}[!htbp]
    \centering
    \caption{List and categorization of earlier adversarial attacks, and of the attacks considered in our evaluation benchmark.}
    \label{table:adv_attacks_categorization}
     \resizebox{\textwidth}{!}{%
    \rowcolors{15}{}{gray!10}
    \begin{tabular}{lllccccllllll}
    \toprule
    \multirow{2}{*}{\textbf{Name}} & \multirow{2}{*}{\textbf{Attack Type}} & \multicolumn{4}{c}{\textbf{Norms}} & \multirow{2}{*}{\textbf{\makecell{Descent\\Direction}}} & \multirow{2}{*}{\textbf{Optimizer}} & \multirow{2}{*}{\textbf{\makecell{Step size ($\alpha$)\\ Scheduler}}}   & \multirow{2}{*}{\textbf{Loss} $L$} & \multirow{2}{*}{\textbf{Init} $\delta_0$}\\
     & & \multicolumn{1}{c}{$\ell_0$} & $\ell_1$ & $\ell_2$ & $\ell_\infty$ & &  & &  & \\
    \midrule
    \biggio~\cite{biggio13-ecml} (2013) & \maxloss &  & \multicolumn{1}{c}{\tcheck} & \multicolumn{1}{c}{\tcheck} & \multicolumn{1}{l}{} & \nochange & \GD & \fixed & $f_y(\vct x; \vct \theta)$ & \originalinit \\
    \szegedy~\cite{szegedy14-iclr-intriguing} (2014) & \minnorm & & &  \multicolumn{1}{c}{}  & \multicolumn{1}{l}{\tcheck} & \nochange & \BFGSB  & \fixed & \crossentropy & \originalinit \\
    \fgsm~\cite{goodfellow15-iclr-explaining} (2015) & \maxloss &  & \multicolumn{1}{l}{} & \multicolumn{1}{l}{} & \multicolumn{1}{c}{\tcheck} & $\linearproj$ & \GD & \fixed & \crossentropy & \originalinit \\ \midrule
    \jsma~\cite{papernot16-sp} (2015) & \minnorm & \multicolumn{1}{c}{\tcheck} & \multicolumn{1}{l}{} & \multicolumn{1}{l}{} & \multicolumn{1}{l}{} & $\linearproj$ & \MomentumGD & \fixed & $z_y(\vct x; \vct \theta)$  & \originalinit \\
    \bim~\cite{kurakin16adversarialexamples} (2016) & \maxloss &  &  &  & \tcheck & \linearproj & \GD & \fixed & \crossentropy & \originalinit \\
    \dfool~\cite{moosavi16-deepfool} (2016) & \minnorm &  &  & \tcheck & & \normalization & \GD & \fixed & \logitloss & \originalinit \\
    \cw~\cite{carlini17-sp} (2017) & \minnorm & \tcheck &  & \tcheck & \tcheck & \nochange & \Adam & \fixed & \logitloss & \originalinit  \\
    \ead~\cite{chen2018ead} (2018) & \minnorm &  & \tcheck & \tcheck & \tcheck & \nochange & \GD & \polynomial & \logitloss & \originalinit  \\
    \pgd~\cite{madry18-iclr} (2018) & \maxloss &  &  & \tcheck & \tcheck & \linearproj & \GD & \fixed & \crossentropy & \originalinit \\
    \bb~\cite{brendel2020accurate} (2019) & \minnorm & \tcheck & \tcheck & \tcheck & \tcheck & \linearproj & \BFGSB & \linear & \logitloss & \adversarialinit \\
    \ddn~\cite{rony2019decoupling} (2019) & \minnorm  &  & & \tcheck & & \normalization & \GD & \cosine & \crossentropy & \originalinit \\
    \pgdlzero~\cite{Croce2019SparseAI} (2019) & \maxloss  & \tcheck &  & &  & \linearproj & \GD & \fixed & \crossentropy & \originalinit \\
    \sfool~\cite{Modas2018SparseFoolAF} (2019) & \minnorm &  & \tcheck & & & \normalization & \texttt{GD$^\star$} & \fixed & \logitloss & \adversarialinit \\
    \tr~\cite{Yao2018TrustRB} (2019) & \minnorm &  & \multicolumn{1}{l}{} & \tcheck & \tcheck & \nochange & \GD & \fixed & \logitloss & \originalinit \\
    \fab~\cite{croce2020minimally} (2020) & \minnorm  &  & \tcheck & \tcheck & \tcheck & \linearproj & \GD & \plateau & \logitloss & \randominit \\
    \apgd~\cite{croce2020reliable} (2020) & \maxloss  &  &  & \tcheck & \tcheck & \linearproj & \MomentumGD & \plateau & \crossentropy/\dlr & \originalinit \\
     \alma~\cite{Rony2020AugmentedLA} (2021) & \minnorm  &  & \tcheck & \tcheck & \multicolumn{1}{l}{} & \nochange & \RMSPropMomentum & \exponential & \dlr & \originalinit  \\
    \apgdlone~\cite{Croce2021MindTB} (2021) & \maxloss  &  & \tcheck &  &  & \linearproj & \MomentumGD & \plateau & \dlr & \originalinit \\ 
    \fmn~\cite{pintor2021fast} (2021) & \minnorm  & \tcheck & \tcheck & \tcheck & \tcheck & \normalization & \GD & \cosine & \logitloss & \anyinit \\
     \pdgd~\cite{Matyasko2021PDPGDPP} (2021) & \minnorm & & & \tcheck & & \linearproj & \Adam & \linear, \exponential & \logitloss & \originalinit \\
     \pdpgd~\cite{Matyasko2021PDPGDPP} (2021) & \minnorm & \multicolumn{1}{c}{\tcheck} & \tcheck & \tcheck & \tcheck & \prox & \Adam & \linear, \exponential & \logitloss & \originalinit \\
    \vfga~\cite{Hajri2020StochasticSA} (2021) & \minnorm  & \multicolumn{1}{c}{\tcheck} & \multicolumn{1}{l}{} & \multicolumn{1}{l}{} & \multicolumn{1}{l}{} & \nochange & \texttt{GD$^\star$} & \fixed & $z_y(\vct x; \vct \theta)$  & \originalinit   \\ 
    \sigmazero~\cite{Cina2024SigmaZero} (2024) & \minnorm  & \multicolumn{1}{c}{\tcheck} & \multicolumn{1}{l}{} & \multicolumn{1}{l}{} & \multicolumn{1}{l}{} & \normalization & \Adam & \cosine & \logitloss & \originalinit   \\ \bottomrule
    \end{tabular}
    }
    \end{table*}

\subsubsection{Minimum-norm vs Fixed-budget Attacks}

Let us assume, without loss of generality, that the input samples lie in a $\con d$-dimensional (bounded) space, \ie $\vct x \in [0, 1]^\con d$, and that their labels are denoted with $y \in \{1, ..., C\}$. Then, the predicted label of a trained model parameterized by $\vct \theta$ can be denoted with $\hat y = f(\vct x, \vct \theta)$, while the confidence value (logit) for class $c$ can be denoted with $f_c(\vct x, \vct \theta)$ and the softmax-rescaled logits with $z_c(\vct x, \vct \theta)$.
The predicted label can thus be computed also as $\hat y = \argmax_c f_c(\vct x, \vct \theta)$.
Under this setting, we argue that finding an adversarial example amounts to solving the following multi-objective optimization:
\begin{eqnarray}
    \label{eq:pareto} \minimize_{\vct \delta} &&  \left ( L(\vct x + \vct \delta, y; \vct \theta) ,  \| \vct \delta \|_p \right ) \, , \\
    \label{eq:constr_pareto}\subjectto && \vct x + \vct \delta \in [0,1]^\con d \, , 
\end{eqnarray}
where $L(\vct x + \vct \delta, y; \vct \theta)$ is a loss defining the misclassification objective, and $\vct \delta$ is the perturbation optimized to find an adversarial example $\vct x^\prime = \vct x+\vct \delta$ within the feasible domain.
The loss function $L: \mathbb{R}^\con d \times \mathbb{R} \to \mathbb{R}$ defines the objective of the attack so that $L$ is large when the input is correctly classified, whereas it is lower when the model predicts a wrong label for $\vct x$.\footnote{For targeted attacks, one can minimize $L(\vct x + \vct \delta, y_t; \vct \theta)$, being $y_t \neq y$ the label of the target class.}
The majority of existing attacks now leverage the Negative Cross-Entropy (\crossentropy) loss, the Difference of Logits (\logitloss)~\cite{carlini17-sp}, or the Difference of Logits Ratio (\dlr)~\cite{croce2020reliable}. 
The second objective in \autoref{eq:pareto} is expressed as a constraint on the size of the perturbation $||\vct \delta||_p$, formulated through the usage of $\ell_p$ norms.
Commonly used perturbation norm constraints are \ellzero, \ellone, \elltwo, \ellinf, that produce respectively sparse to increasingly dense perturbations.
The constraint in \autoref{eq:constr_pareto} is a box constraint that ensures the sample remains within the input space of the model, \ie $\vct x + \vct \delta \in [0, 1]^\con d$. 

The optimization problem expressed in \autoref{eq:pareto} presents an inherent tradeoff: minimizing $L$ favors the computation of adversarial examples with large misclassification confidence, but also a large perturbation size, whereas minimizing $\| \vct \delta \|_p$ penalizes larger perturbations (in the given $\ell_p$ norm) at the expense of decreasing the misclassification confidence.
%Multi-objective problems like \autoref{eq:pareto} can be solved by establishing a trade-off between the given objectives along the Pareto frontier by optimizing one objective and using the other as a constraint.
Consequently, we can find two main families of attacks, where one aims at finding the inputs that cause the maximum error within a given perturbation budget (\maxloss), and the counterpart that searches for the smallest perturbation needed to achieve misclassification (\minnorm).

\myparagraph{Fixed-budget Attacks.}  
We call a first group fixed-budget attacks (\maxloss), which minimize the loss and set the perturbation size as the constraint. They optimize the following problem:
\begin{eqnarray}
\label{eq:obj_max_conf} \minimize_{\vct \delta}  && L(\vct x + \vct \delta, y, \vct \theta) \, , \\
\label{eq:constr_max_conf}	\subjectto && \|\vct \delta \|_{p} \leq \epsilon \, ,  \\ 
\label{eq:bounds_max_conf}	&&  \vct x + \vct \delta \in [0,1]^\con d \, ,
\end{eqnarray}

where $\| \cdot\|_{p}$ indicates the $\ell_p$-norm operator. 
The loss $L$ in the objective of \autoref{eq:obj_max_conf} is a loss function approximating the classification outcome, defined accordingly to the goal of the attack, \ie untargeted or targeted misclassification.
For example, this group of attacks includes Projected Gradient Descent (\pgd)~\cite{madry18-iclr}. 
%, which is formulated as $\min_{\vct \delta} L(\vct x + \vct \delta, y, \vct \theta)$ s.t. $\| \vct \delta \|_p \leq \epsilon$.

\myparagraph{Minimum-norm Attacks.} %On the other hand, minimum-norm 
these attacks (\minnorm) minimize the size of the perturbation and set the misclassification on the model as a constraint. 
They are formulated as follows:
\begin{eqnarray}
    \label{eq:obj_min_distance}	\minimize_{\vct \delta}  && \|\vct \delta \|_{p}  \\
    \label{eq:constr_min_distance}	\subjectto  &&  f(\vct x + \vct \delta, \vct \theta) \neq f(\vct x, \vct \theta)\, , \\
    \label{eq:bounds_min_distance}	&& \vct x + \vct \delta \in [0,1]^\con d \, 
 ,
\end{eqnarray}
where $|| \cdot||_{p}$ indicates the $\ell_p$-norm operator. 
However, this problem cannot be solved directly by gradient descent since the misclassification constraint \eqref{eq:constr_min_distance} is not differentiable.

There are two ways to solve this problem.
The first solution adopts the \maxloss formulation for different values of $\epsilon$, by applying heuristics to minimize the norm of the perturbation (like enlarging or shrinking $\epsilon$ during the computations, as done by Decoupling-Direction-Norm (\ddn)~\cite{rony2019decoupling}, and the Fast Minimum-Norm (\fmn)~\cite{pintor2021fast} attacks).
The other solution consists of transforming the constrained problem into an unconstrained one, by using a differentiable relaxation of the constraint~\eqref{eq:constr_min_distance}, \eg, the difference between the output score of the original class $y$ and the scores of the other classes, and adding it to the objective as a penalty component, with an appropriate trade-off parameter.
For instance, the Carlini-Wagner attack (\cw) \cite{carlini17-sp} implements the following objective: $\min_{\vct \delta} \| \vct \delta \|_p + c \cdot \min(L(\vct x + \vct \delta, y , \vct \theta), -\kappa)$, where $c$ controls the trade-off between the misclassification objective and the perturbation size.
However, these penalty methods are slow in practice ($c$ requires a search). 
Thus, an Augmented Lagrangian Method for Adversarial 
(\alma) attacks \cite{Rony2020AugmentedLA} has been proposed to adaptively adjust the trade-off between the norm minimization objective and the misclassification constraint, by leveraging penalty-Lagrangian functions.

In contrast to \maxloss attacks, which maximize confidence for predicting a wrong class within a given perturbation budget, \minnorm attacks aim at finding the closest adversarial example to each input. This requires solving a more complex problem, as it amounts not only to finding a valid adversarial example, but also to minimizing its perturbation size~\cite{Rony2020AugmentedLA}.

\begin{algorithm}[t]
 \SetKwInOut{Input}{Input}
    \SetKwInOut{Output}{Output}
    \SetKwComment{Comment}{$\triangleright$\ }{}
    \DontPrintSemicolon
	\caption{Generalized Attack Algorithm}
	\label{algo:unified_attack_algorithm}
   \Input{$\vct x$, the input sample; $y$, the class label; \stepsize, the initial step size; $\vct \theta$, target model; and \numberofsteps, the number of iterations.}
	\Output{The adversarial example $\vct x_{\rm adv}$.}
     $\vct \delta_{0} \gets \textcolor{orange}{\texttt{init}}(\vct x) $\label{line:init}\Comment*[r]
     {\textcolor{orange}{initialization}}
    $\vct \delta^\star \gets \vct \delta_0$, $\alpha_{0}=\alpha$ \\
    \For {$\stepindex = 1, \ldots, \numberofsteps$} 
	    {$\vct g \gets \nabla_{\vct \delta} \textcolor{blue}{L}(\vct x +\vct \delta_{k-1}, y,  \vct \theta)$ \Comment*[r]{\textcolor{blue}{loss} gradient}\label{line:gradient}
    $\vct g \gets \textcolor{violet}{\texttt{direction}}(\vct g, \stepsize_\stepindex)$\label{line:gradient_transform}\Comment*[r]{\textcolor{violet}{descent direction}}
        $\vct \delta_{k} \gets$ \textcolor{cyan}{\texttt{optim}}($\vct x, \vct \delta_{k-1}, \vct g)$ \label{line:opt_step} \Comment*[r]{\textcolor{cyan}{optimizer} (proj.)}
        %$\vct \delta_{k} \gets \vct \delta_{k-1} -  \Pi_{\alpha_k}(\vct g)$ \\
        %$\Pi(\vct x +\vct \delta_k) $ \\
        
	   $\stepsize_{\stepindex} \gets \textcolor{red}{\texttt{scheduler}}(\stepsize_{0}, \stepindex, \numberofsteps)$ \Comment*[r]{\textcolor{red}{scheduler}} \label{line:gamma_decay}
        %$\alpha_{\stepindex} \gets \gamma_\stepindex \alpha$ \Comment*[r]{scheduler step}\label{line:step_decay}
        %$\vct \delta_k \gets \Pi_\Delta (\vct x_0, \vct \delta_k)$ \label{line:project} \Comment*[r]{projection onto $\Delta$}
    }

 $\vct \delta^\star \gets \texttt{best}(\vct \delta_0, ... \vct \delta_\numberofsteps$)\label{line:return} \Comment*[r]{best solution}
	\bfseries return $\vct x_{\rm adv} = \vct x + \vct \delta^\star$ 
\end{algorithm}

\myparagraph{Solution Algorithm.} We describe here a generalized attack, given as \Cref{algo:unified_attack_algorithm}, which encompasses the main steps performed by most of the \maxloss and \minnorm attacks. 
The attack starts by initializing the perturbation (\cref{line:init}), and then iterates $K$ times.
In each iteration, the attack computes the gradient of the loss function (\cref{line:gradient}), which is processed accordingly to match norm constraints (\cref{line:gradient_transform}), and then it is used to tune the perturbation (\cref{line:opt_step}).
Then, attacks might update their hyper-parameters (\cref{line:gamma_decay}). 
%before enforcing the constraints expressed by $\Delta$ (\cref{line:project}).
Once all the iterations have been consumed, the attack returns the best perturbation computed so far (\cref{line:return}).
While these steps are general, we now detail 
the function and the possible choices of each component 
used in \Cref{algo:unified_attack_algorithm}.
%Each attack implements a distinct strategy, aligning with a specific choice of the components detailed within this section.

\subsubsection{Loss Functions}
Typically, the loss $L$ in \autoref{eq:pareto} for a gradient-based attack (\cref{line:gradient}) is defined as $L: \mathbb{R}^\con d \times \mathbb{R} \to \mathbb{R}$.
While early attacks used directly the $y$-th logit output of the models ($f_y(\vct x; \vct \theta)$)~\cite{biggio13-ecml, szegedy14-iclr-intriguing} or the $y$-th softmax output ($z_y(\vct x; \vct \theta)$)~\cite{papernot16-sp}, the majority of existing attacks now leverage the Negative Cross-Entropy (\crossentropy) loss, the Difference of Logits (\logitloss)~\cite{carlini17-sp}, or the Difference of Logits Ratio (\dlr)~\cite{croce2020reliable}. 
%As stated in \autoref{eq:pareto}, all these losses are defined so that their minimization leads to the adversarial region.

\myparagraph{Logit and Softmax Loss.} 
Earlier attacks, as the one proposed by Biggio~\etal~\cite{biggio13-ecml}, and Papernot~\etal~\cite{papernot16-sp} directly optimize the $y$-th output of the model $f_y(\vct x; \vct \theta)$, or its softmax-scaled value $z_y(\vct x; \vct \theta)$. The softmax outputs have recently been used also in the Voting Folded Gaussian Attack~\cite{Hajri2020StochasticSA}.

\myparagraph{Negative Cross-entropy Loss (\crossentropy).} Firstly used by Szegedy \etal~\cite{szegedy14-iclr-intriguing}, this loss is computed as
        $L(\vct x, y; \vct \theta) =\log(z_y(\vct x; \vct \theta)).$
This is basically the standard cross-entropy loss multiplied by~$-1$ as now the goal is to \textit{increase} the error of the model.
For a targeted attack, it is sufficient to use the target label $y_t$ instead of the true label $y$, and flip the sign.

\myparagraph{Difference of Logits Loss (\logitloss).} Introduced by Carlini and Wagner~\cite{carlini17-sp} in the popular attack that brings their name, this loss is directly computed with the logits, \ie the outputs of the model:
%\begin{equation}\label{eq:cw_loss}
$L(\vct x, y; \vct \theta) =  f_{y}(\vct x; \vct \theta) - \max_{j \neq y}f_{j}(\vct x; \vct \theta) \, .$
%\end{equation}
Assuming the classifier assigns higher scores to the correct class, the loss function takes on negative values when $\vct x$ becomes adversarial.
As for the previous case, this loss can become targeted if the score $ f_{t}(\vct x; \vct \theta)$ is used instead of the score for the original class, and the sign of the loss is swapped, \ie the objective becomes maximizing the logit of the target class.
It is worth noting that setting this loss equal to zero means finding the decision boundary, while imposing an offset means enforcing a margin of misclassification confidence on the prediction.
For this reason, Carlini \etal~\cite{carlini17-sp} introduce the misclassification margin in the loss, \ie $\min(L(\vct x + \vct \delta, y; \vct \theta), -\kappa)$, where $\kappa$ represents the minimum distance required between the two scores.

\myparagraph{Difference of Logit Ratio Loss (\dlr).} Introduced by Croce~\etal~\cite{croce2020reliable}, this loss function is both shift and rescaling invariant to the outputs of the model.
This is obtained by using the Logit Difference Loss and dividing it by a scaling factor computed on the logits themselves as follows:
\begin{equation*}\label{eq:dlr_loss}
        L(\vct x, y; \vct \theta) = \frac{f_{y}(\vct x; \vct \theta) - \max_{j \neq c}f_{j}(\vct x; \vct \theta)}{f_{\pi_1}(\vct x; \vct \theta) - f_{\pi_3}(\vct x; \vct \theta)},
\end{equation*}
where $f_{\pi_1} (\vct x; \vct \theta) \geq \ldots \geq f_{\pi_c}(\vct x; \vct \theta)$ denote the logits sorted in decreasing order. The shift invariance is achieved by applying a normalizing factor composed of a difference of top-ranking logits in the denominator.

\subsubsection{Initialization Strategies}

Some attacks perform a custom initialization to favor a better exploration of the loss landscape. 
Initialization can be modeled as transformations 
$i: \mathbb{R}^\con d \to \mathbb{R}^\con d$, and return a valid sample in the feasible domain $\Delta$ (\cref{line:init}).
The baseline option is to start the attack from the original point (\originalinit). 
Another option is choosing a random initialization (\randominit), which sets the initial estimate of $\vct \delta_0$ to be a random perturbation within the constraints of the optimization problem, as done by \fab~\cite{croce2020minimally}. 
Note that some attacks may also internally run the attack starting from multiple random restarts and take the best perturbation out of all trials to improve the optimization results~\cite{Croce2019SparseAI}.
Other attacks, like \bb~\cite{brendel2020accurate} and optionally \fmn~\cite{pintor2021fast}, can be initialized as a sample belonging to a specific target class (\adversarialinit), and minimize the perturbation by getting closer and closer to $\vct x$ during the iterations.

\subsubsection{Descent Directions}

To speed-up the optimization, attacks use different  strategies that modify the gradient in each iteration before passing it to the optimizer (\cref{line:gradient_transform}).
We identify four main strategies to define appropriate descent directions:

\mylist{1.} Gradient (\nochange), which uses the gradient $\vct g$ \textit{as is};

\mylist{2.}  Normalization (\normalization), which keeps the direction of $\vct g$ but rescales its norm to be proportional to the step size $\stepsize_\stepindex$ in the current iteration, \ie, $\vct g^{\prime} = \frac{\stepsize_\stepindex \vct g}{s}$, where the scaling factor is often set as $s=\| \vct g \|_p$;

\mylist{3.}  Projection (\linearproj), which sets the direction by maximizing the scalar product with the gradient $\vct g$ over an $\stepsize_\stepindex$-sized $\ell_p$ ball, as $\vct %g^{\prime} \in \underset{\parallel \vct v \parallel_p \leq \stepsize_\stepindex}{\argmax } \, \vct v^\top \vct g$;
g^{\prime} \in \argmax_{\parallel \vct v \parallel_p \leq \stepsize_\stepindex} \, \vct v^\top \vct g$;\footnote{This amounts to maximizing the linear approximation of the loss function $L(\vct x + \vct v, y, \vct \theta) \approxeq L(\vct x, y, \vct \theta) + \vct v^T \nabla L(\vct x, y, \vct \theta)$ over an $\stepsize_\stepindex$-sized $\ell_p$ ball.}

\mylist{4.} Proximal (\prox), which uses the proximal gradient~\cite{parikh2014proximal}.

PGD-based attacks all use \linearproj, as for $p \in \{1, 2, \infty\}$ the solution can be efficiently computed in closed form. 
For $p=1$, the maximum is achieved by taking the  components of $\vct g$ with maximum absolute values and setting them to $\pm \stepsize_\stepindex$, according to their sign. 
In practice, this leads to poor performance when combined with the box constraint in \autoref{eq:bounds_min_distance}, as it results in updating only one component in each iteration.
Reformulations of this update generally include the box constraint in the maximization, \eg, in $\ell_1$-\apgd~\cite{croce2020reliable}, which update the components exhibiting the largest absolute values at once, up to the box limits, until an \ellone norm of $\stepsize_\stepindex$ is achieved.
For $p=2$, the maximum is achieved when $\vct g^\prime = \stepsize_\stepindex\frac{\vct g}{\|\vct g\|_2}$, which is practically equivalent to \normalization.
For $p=\infty$, the maximum is achieved by setting $g^\prime = \sign(\vct g)$, resulting in a dense update of all components of $\vct \delta_\stepindex$ as in the \ellinf-\pgd attack~\cite{madry18-iclr}.

\subsubsection{Optimizers}
This attack component applies the update on the current perturbation, producing a new perturbation $\vct \delta_\stepindex$. 
Optimizers are specific algorithms that implement this update, $u: \mathbb{R}^\con d \mapsto \mathbb{R}^\con d$, based on the computed gradient and a specific strategy (\cref{line:opt_step}) and return a perturbation vector of the same dimension as the input . 
Existing gradient-based adversarial attacks use different variants of Gradient Descent (\GD), sometimes with a diagonal metric to scale different axes of the space (\eg Adam (\Adam)) or introducing a momentum term to avoid vanishing gradient issues (\eg Momentum (\MomentumGD)). 
Alternatively, they can use adaptive strategies where the learning rate changes over time (\eg RMSprop with momentum (\RMSPropMomentum)) or second-order derivative methods (\eg \BFGSB). Optimizers can also be combined together as in attacks that integrate linear solvers with other gradient-based sub-routine attacks (\GDLinearSolv).
Finally, the optimizer step might include a final projection operation that ensures the produced update $\vct x + \delta_\stepindex$ is in the feasible domain. 
Specifically, it takes into account the box constraint in~\autoref{eq:pareto} and eventually the $\pertsize$ bound in \autoref{eq:constr_max_conf} for the case of \maxloss attacks.

\subsubsection{Step Size Schedulers}
Some attacks, including most of the \maxloss attacks, use a fixed step size (\fixed).
However, as well known in optimization theory, when using \GD, decreasing the step size usually leads to better convergence results. 
Thus, dedicated schedulers can control the optimization process. We denote them as a function $h: \mathbb{R} \mapsto \mathbb{R}$, that dynamically updates the step size $\stepsize$ (\cref{line:gamma_decay}) and tune the decay to guarantee better convergence.    
Indeed, many attacks, especially the \minnorm, reduce the step size along the iterations, shrinking the trust region of the linear approximation (thus, the step size) to refine the solution with smaller updates as they approach the boundary. 
One common strategy is to use a linear step size decay (\linear), in which the step size is multiplied by a fixed amount $\gamma<1$ at each step. 
Another popular scheduler is the Cosine Annealing (\cosine)~\cite{loshchilov2017sgdr}, which decays the step size gradually from a maximum value of $\stepsize$ to a minimum of $\stepsize_\numberofsteps$. 
Other alternatives are exponential (\exponential) or polynomial (\polynomial) step size decay, where the decay is controlled by an exponential descent or a specified polynomial, respectively. 
As another strategy, some attacks adapt the step size depending on the loss behavior over a span of iterations. 
In particular, when the loss plateaus for a specified number of steps, this scheduler reduces the step size by a defined factor (\plateau).
While these attacks are often called \textit{adaptive}, the term adaptive is already used in the State of the Art of adversarial attacks for denoting attacks that are customized to break a specific defense
~\cite{tramer2020adaptive}.

\subsection{Limitations of Current Evaluations}

In current evaluations and comparisons of gradient-based attacks, there are several limitations that we aim to address with our proposed framework. 
These evaluations are often conducted independently in each research paper, increasing the risk of overfitting the metrics proposed within that study and hindering reproducibility. Specifically:

\mylist{1.} Attacks are not re-evaluated against recent robust models; %(\autoref{sec:testing_attacks});

\mylist{2.} \maxloss are compared for arbitrary values of \pertsize, whereas \minnorm generally rank attacks with the median size of perturbation, making the comparison between the two categories difficult;% (\autoref{sec:optimality});

\mylist{3.} Considered metrics are not combinable across models to reflect a global performance of the attacks ;%(\autoref{sec:optimality});

\mylist{4.} Use different datasets or subsets of points, hard to re-create;% (\autoref{sec:implementation_benchmark});

\mylist{5.} Provide attacks with different computational budgets;%(\autoref{sec:implementation_benchmark}). %First, some attacks dynamically optimize their hyperparameters using sub-routines, thus the number of steps is not indicative~\cite{carlini17-sp}. Moreover, some attacks exploit additional model propagations (\eg \cite{croce2020minimally} to find the closest decision boundary \wrt a linear approximation)...

\mylist{6.} Later re-implementations of published attacks might deviate from the original ones, and these differences are often not taken into account; %(\autoref{sec:exp_results}); and

\mylist{7.} Results are not shared, and when new attacks emerge, evaluations have to be re-run completely.%(\autoref{sec:implementation_benchmark}).

We address all these limitations with \ab, described in \autoref{sec:attackbench}, providing a more comprehensive and reliable evaluation framework for adversarial attacks.
